# Supplementary material for: Enhancing Network Resilience through Machine Learning-powered Graph Combinatorial Optimization: Applications in Cyber Defense and Information Diffusion
Source: arXiv:2310.10667 source file (2023-09-22)
Supplement: Supplementary file 1 [file AppendixTemplate.tex]

% Appendix Template

\chapter{Appendix Title Here} % Main appendix title

\label{AppendixX} % Change X to a consecutive letter; for referencing this appendix elsewhere, use \ref{AppendixX}

Write your Appendix content here.
